# Supplementary material for: Motion Estimation for Fisheye Video With an Application to Temporal Resolution Enhancement
Source: arXiv:2303.00433 source file (2023-03-01)
Supplement: Supplementary file 1 [file myappendix.tex]

Everything below is misc info. Delete!

\subsection{Approximated Models}

Actual lenses rarely follow an exact mathematical model due to manufacturing inaccuracies.
For this reason, a camera calibration is performed to get information on the projection function employed by the lens.
In this context, polynomial approximations are often used as they are able to describe the exact projections fairly well.
A simple approximation is given by a polynomial of 3rd order, which only needs two parameters or coefficients:
\begin{equation}
r_d = k_1\theta + k_2\theta^3
\end{equation}
For equisolid: $k_1 = f$, $k_2 \approx -0.0727$.\\
For equidistant: $k_1 = f$, $k_2 = 0$.

One-parameter model by Devernay and Faugeras~\cite{devernay2001straightlines}:
\begin{align}
r_d &= \frac{1}{\omega}\arctan\left(2r_u\tan\left(\frac{\omega}{2}\right)\right) \\
\mathrm{and\quad} r_u &= \frac{\tan\left(r_d\omega\right)}{2\tan\left(\frac{\omega}{2}\right)}
\end{align}

\subsection{World to image etc.}

Some basics (applies to 2D and 3D).\\
Dot product/inner product $\langle\cdot,\cdot\rangle$:
\begin{equation}
\boldsymbol{a}\cdot \boldsymbol{b} = \langle\boldsymbol{a},\boldsymbol{b}\rangle = a_1b_1+a_2b_2+a_3b_3
\end{equation}
Magnitude $\lvert\cdot\rvert$:
\begin{equation}
\lvert \boldsymbol{a} \rvert = \sqrt{a_1^2+a_2^2+a_3^2}
\end{equation}
Angle between two vectors:
\begin{equation}
\cos \alpha = \frac{\langle\boldsymbol{a},\boldsymbol{b}\rangle}{\lvert\boldsymbol{a}\rvert\lvert\boldsymbol{b}\rvert} 
\end{equation}

\begin{figure}[t]
%\small
\centering
\centerline{\includegraphics[width=1.0\columnwidth]{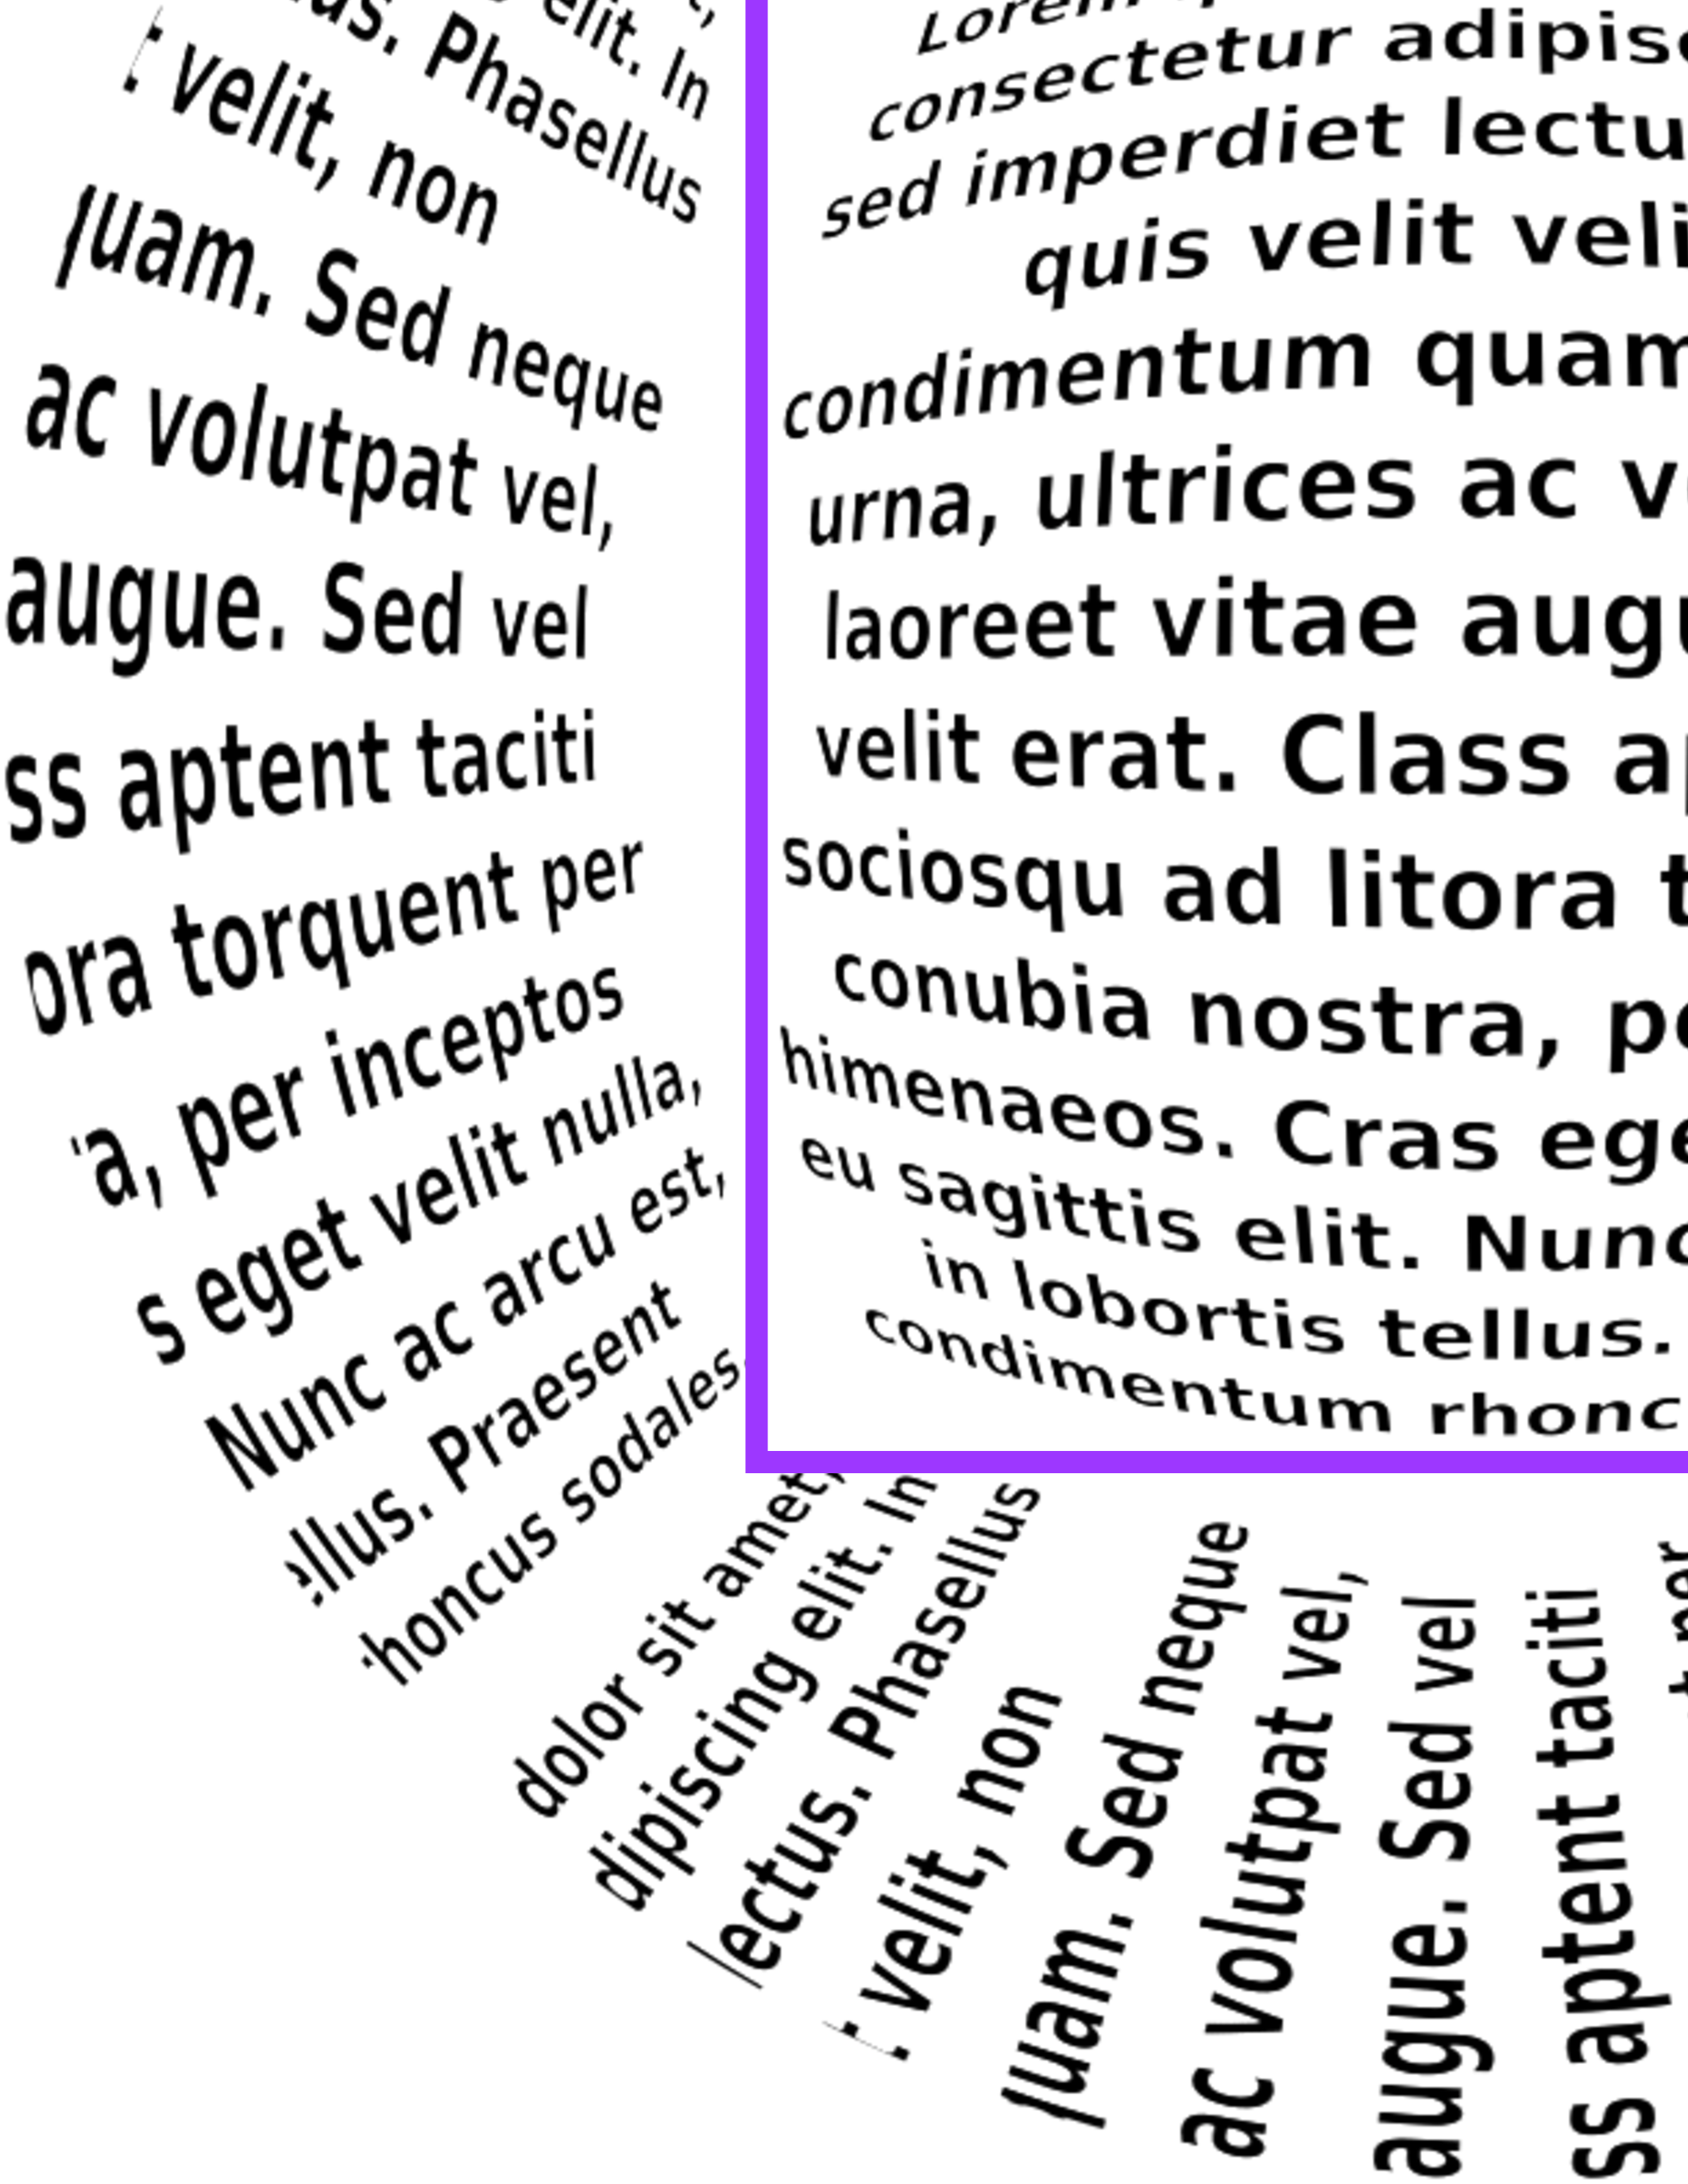}}
%\vspace{-0.2cm}
\caption{TODO.}
\label{fig:fovmotion}
%\vspace{-0.6cm}
\end{figure}

\begin{figure}[t]
%\small
\centering
\centerline{\includegraphics[width=1.0\columnwidth]{figures/blockmatchingexmp}}
%\vspace{-0.2cm}
\caption{PLACEHOLDER -- Fisheye motion image as motivation. Include arrow to indicate motion. Change images and colors and maybe add perspective case.}
%\label{fig:pinhole}
%\vspace{-0.6cm}
\end{figure}

\begin{figure}[t]
\centering
\input{figures/radiusprojection}
\caption{Blue: Absolute distance to image center on perspective grid after employing~(\ref{eq:backward}) on equisolid fisheye grid, cf.~(\ref{eq:pinhole}). Red: linear mapping $r_e = r_e$ as a reference. Dashed asymptote: $r_\text{e}(\theta = \pi/2)\approx 532$ and $r_\text{p}(\pi/2) = \infty$.}
\label{fig:radiusprojection}
\end{figure}

\subsection{Perspective-to-Fisheye Mapping}

Given a point $\boldsymbol{P}=(X,Y,Z)^T$ in a three-dimensional Cartesian coordinate system, this point shall be projected via the pinhole model.
The pinhole is located at the origin $(0,0,0)^T$ of the coordinate system as shown in Fig.~\ref{fig:pinhole}.
The projected 2D point on the perspective image plane is (indirectly) obtained by:
\begin{equation}
\lvert\boldsymbol{P}_{\text{p}}\rvert = r_{\text{p}}= f \tan{\theta}\:.
\end{equation}
Here, $\theta$ is the angle between the vector $\boldsymbol{P}$ and the Z-axis, which corresponds to the incident angle of light measured against the optical axis. The optical axis coincides with the Z-axis.
In the following, $\boldsymbol{Z}$ is the unit vector $(0,0,1)^T$, with $\lvert \boldsymbol{Z} \rvert = 1$, and $\lvert \boldsymbol{P}\rvert = r$.
\begin{equation}
\theta = \arccos{\left( \frac{ \langle\boldsymbol{P},\boldsymbol{Z}\rangle }{ \lvert \boldsymbol{P} \rvert \lvert \boldsymbol{Z} \rvert } \right)} = \arccos{\left( \frac{z}{r} \right)}
\end{equation}

The following is derived from~\cite{jin2015warpedfisheye}, which did not use real fisheye images.

A typical notation for images could be as follows.
Given an image $\mathbf{S}$ of size $M\times N$ pixels, where $M$ is the width and $N$ is the height of the image, let the single discrete image pixels be denoted as $s[m,n]$, with $0\leq m<M$ and $0\leq n<N$.
The image center is given by the tuple $(\lfloor M/2\rfloor, \lfloor N/2\rfloor )$, the corresponding intensity value thus is $s[\lfloor M/2\rfloor, \lfloor N/2\rfloor ]$. (In MATLAB, $\lceil\cdot \rceil$ is used as counting starts from 1 instead of 0.)

Assuming now a Cartesian grid with coordinates $x$ and $y$, let this grid be centered around the image center, i.\,e., the image center $(\lfloor M/2\rfloor, \lfloor N/2\rfloor )$ is located at position $x=0$ and $y=0$.
In other words, we assume that the image $\mathbf{S}$ is shifted such that its center is located at the center of the Cartesian grid.
We now denote the single discrete pixels as $s[x,y]$, with $-\lfloor M/2\rfloor \leq x < \lceil M/2\rceil$ and $-\lfloor N/2\rfloor \leq y < \lceil N/2\rceil$.
The tuples $(x,y)$ denote the respective pixel coordinates or pixel positions.
In the following, only the Cartesian notation $(x,y)$ is used.
From here on, $(0,0)$ denotes the image center.

The Euclidean distance of a given point $\boldsymbol P_{\text{p}}$ located at position $(x,y)$ on the Cartesian grid to the center $(0,0)$ is obtained by
\begin{equation}
r_{\text{p}} = \sqrt{x^2 + y^2}\quad .
\end{equation}
$r_{\text{p}}$ denotes the Euclidean distance or radius in the conventional perspective representation, i.\,e., the underlying imaging model is the pinhole model.
Correspondingly, the polar coordinates of $\boldsymbol P_{\text{p}}$ are expressed as ($r_{\text{p}},\phi$). The projection onto the perspective image plane is visualized in the top part of Fig.~\ref{fig:persp2equisolid}.

If we deal with fisheye images, different models are made use of.
One such model is the equisolid angle model.
Another one is the equidistant model.
We will now focus on the equisolid model and derive the warping functions.

In the fisheye representation, here the equisolid fisheye image, we use the coordinates $u$ and $v$ to form the image grid.
Note that in this representation, we do not necessarily deal with integer values (as was the case for $x$ and $y$).
The distance to the center is obtained by
\begin{equation}
r_{\text{e}} = \sqrt{u^2 + v^2}\quad ,
\end{equation}
where, again, the whole coordinate grid is centered at the image center or optical axis.
The polar coordinates are thus given by $(r_{\text{e}},\phi)$.
Note that the polar angle $\phi$ is the same as in the perspective projection.
The equisolid image plane is visualized in the middle part of Fig.~\ref{fig:persp2equisolid}.
Since the equisolid fisheye model can map a larger FOV onto an image plane of given dimensions (dependent on the camera sensor dimensions), a light ray with incident angle $\theta$ is projected closer to the image center than was the case for the perspective projection.
Given $\theta$ and $f$, this means that $r_{\text{e}}<r_{\text{p}}$ is always true.
This fact can also be derived from Fig.~\ref{fig:projections}.

The bottom part of Fig.~\ref{fig:persp2equisolid} shows a merged top-down view of both the perspective and the equisolid image planes.
Using similar triangles (highlighted in red and green), the following ratios are equal:
\begin{equation}
\frac{r_{\text{p}}}{r_{\text{e}}} = \frac{x}{u} = \frac{y}{v}\: .
\end{equation}

\begin{figure}[t]
%\small
\centering
\psfrag{x}[lB][lB]{$x$}
\psfrag{y}[lB][lB]{$y$}
\psfrag{u}[lB][lB]{$u$}
\psfrag{v}[lB][lB]{$v$}
\psfrag{o}[lB][lB]{$\phi$}
\psfrag{p}[lB][lB]{{\color[rgb]{0.6,0.3,0.3}perspective plane}}
\psfrag{q}[lB][lB]{{\color[rgb]{0.3,0.6,0.3}equisolid plane}}
\psfrag{s}[lB][lB]{{\color[rgb]{0.3,0.3,0.3}similar triangles}}
\psfrag{a}[cB][cB]{{\color[rgb]{0.3,0.3,0.3}optical axis}}
\psfrag{r1}[lB][lB]{$r_{\text{p}}$}
\psfrag{r2}[lB][lB]{$r_{\text{e}}$}
\psfrag{z1}[lB][lB]{{\color[rgb]{0.6,0.3,0.3}$\boldsymbol{P}_{\text{p}}$}}
\psfrag{z2}[lB][lB]{{\color[rgb]{0.3,0.6,0.3}$\boldsymbol{P}_{\text{e}}$}}
\centerline{\includegraphics[width=\columnwidth]{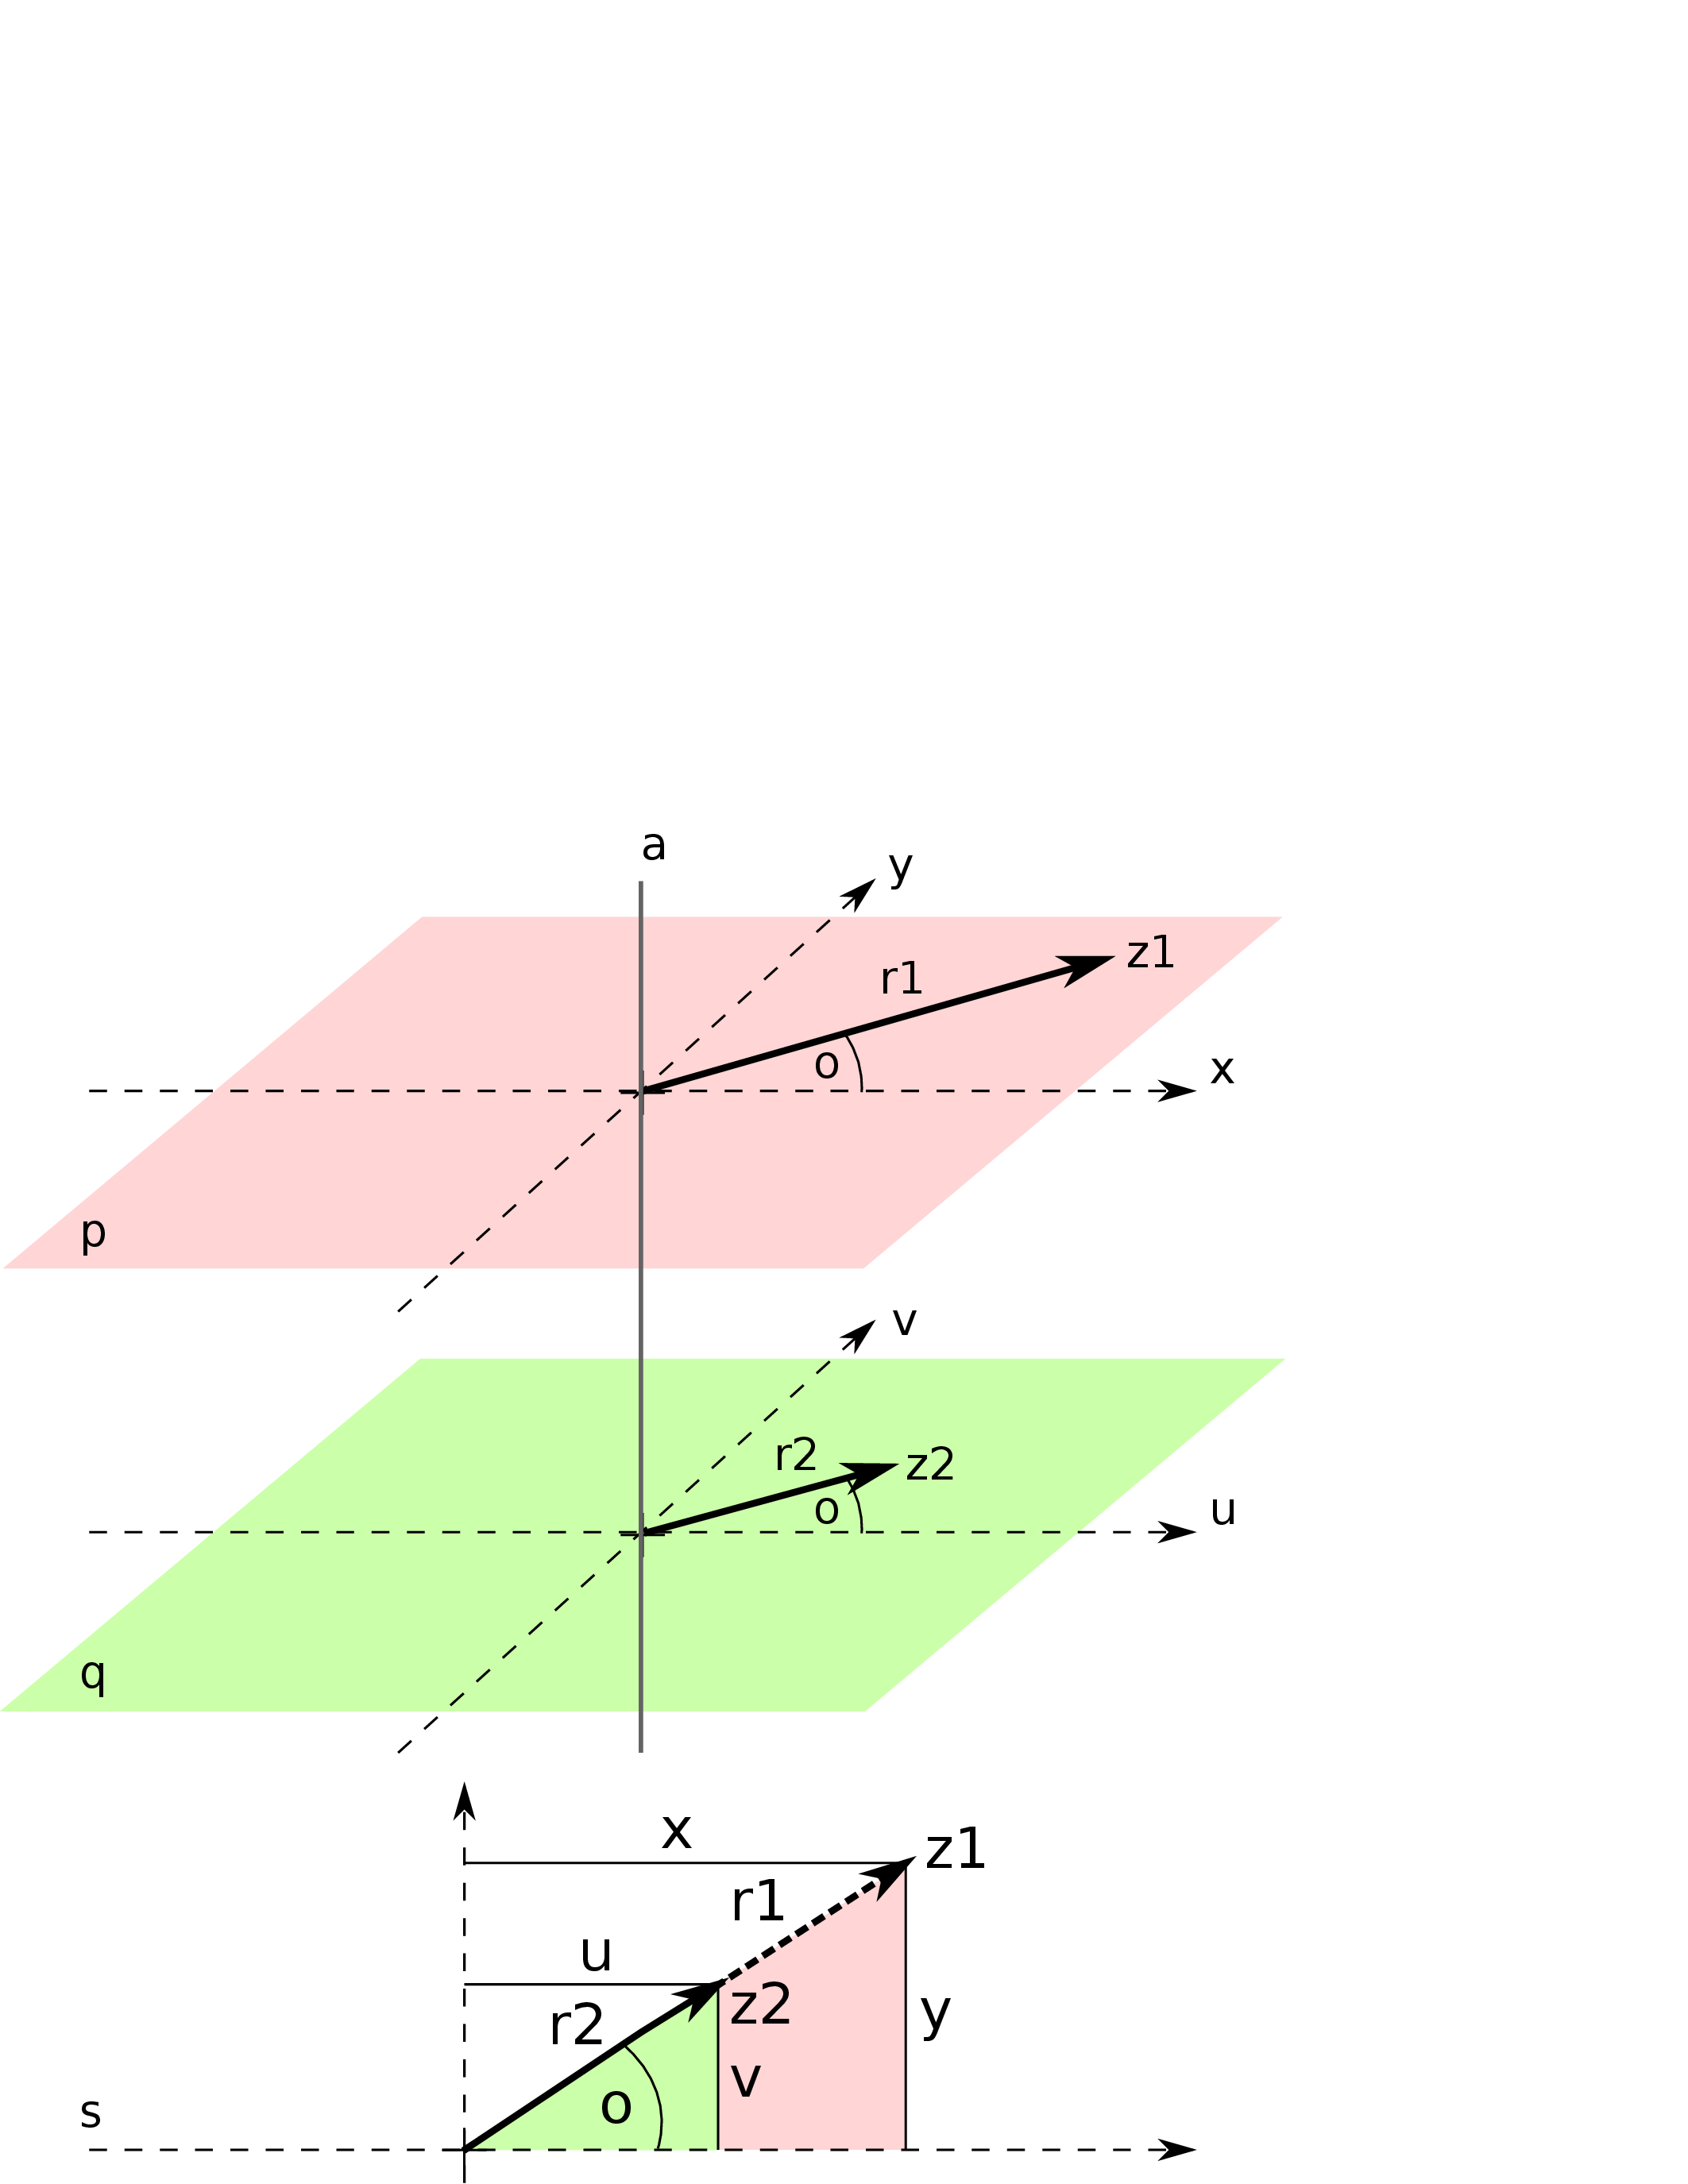}}
%\vspace{-0.2cm}
\caption{Given a point $\boldsymbol P$ in three-dimensional space, this point is projected onto $\boldsymbol P_{\text{p}}$ by perspective projection and onto $\boldsymbol P_{\text{e}}$ by equisolid projection. The relation between both projections can be derived using similar triangles.}
\label{fig:persp2equisolid}
%\vspace{-0.6cm}
\end{figure}

Using these relationships, a mapping from the perspective coordinates $(x,y)$ to the equisolid fisheye coordinates $(u,v)$ can be derived:
\begin{align}
%\begin{pmatrix}a\\b\end{pmatrix}
u &= x \frac{r_{\text{e}}}{r_{\text{p}}} = x \frac{2f}{\sqrt{x^2 + y^2}} \sin\left(\frac{1}{2} \arctan\left(\frac{\sqrt{x^2 + y^2}}{f} \right) \right) \\
v &= y \frac{r_{\text{e}}}{r_{\text{p}}} = y \frac{2f}{\sqrt{x^2 + y^2}} \sin\left(\frac{1}{2} \arctan\left(\frac{\sqrt{x^2 + y^2}}{f} \right) \right)
\end{align}
Please note that the equations above are not defined for $x = y = 0$; in this case the mapping $u = x = 0$ and $v = y = 0$ applies.
With this mapping, the relationship between the perspective and the fisheye domain is expressed. 
The inverse mapping is analogously given by:
\begin{align}
x &= u \frac{r_{\text{p}}}{r_{\text{e}}} = u \frac{f}{\sqrt{u^2 + v^2}} \tan\left(2\arcsin\left(\frac{\sqrt{u^2 + v^2}}{2f}\right)\right) \\
y &= v \frac{r_{\text{p}}}{r_{\text{e}}} = v \frac{f}{\sqrt{u^2 + v^2}} \tan\left(2\arcsin\left(\frac{\sqrt{u^2 + v^2}}{2f}\right)\right)
\end{align}
Again, if $ u = v = 0$, the mapping $x = u = 0$ and $y = v = 0$ applies.

\begin{figure}[t] % CarparkA frame 80
%\small
\centering
\centerline{\includegraphics[width=1.0\columnwidth]{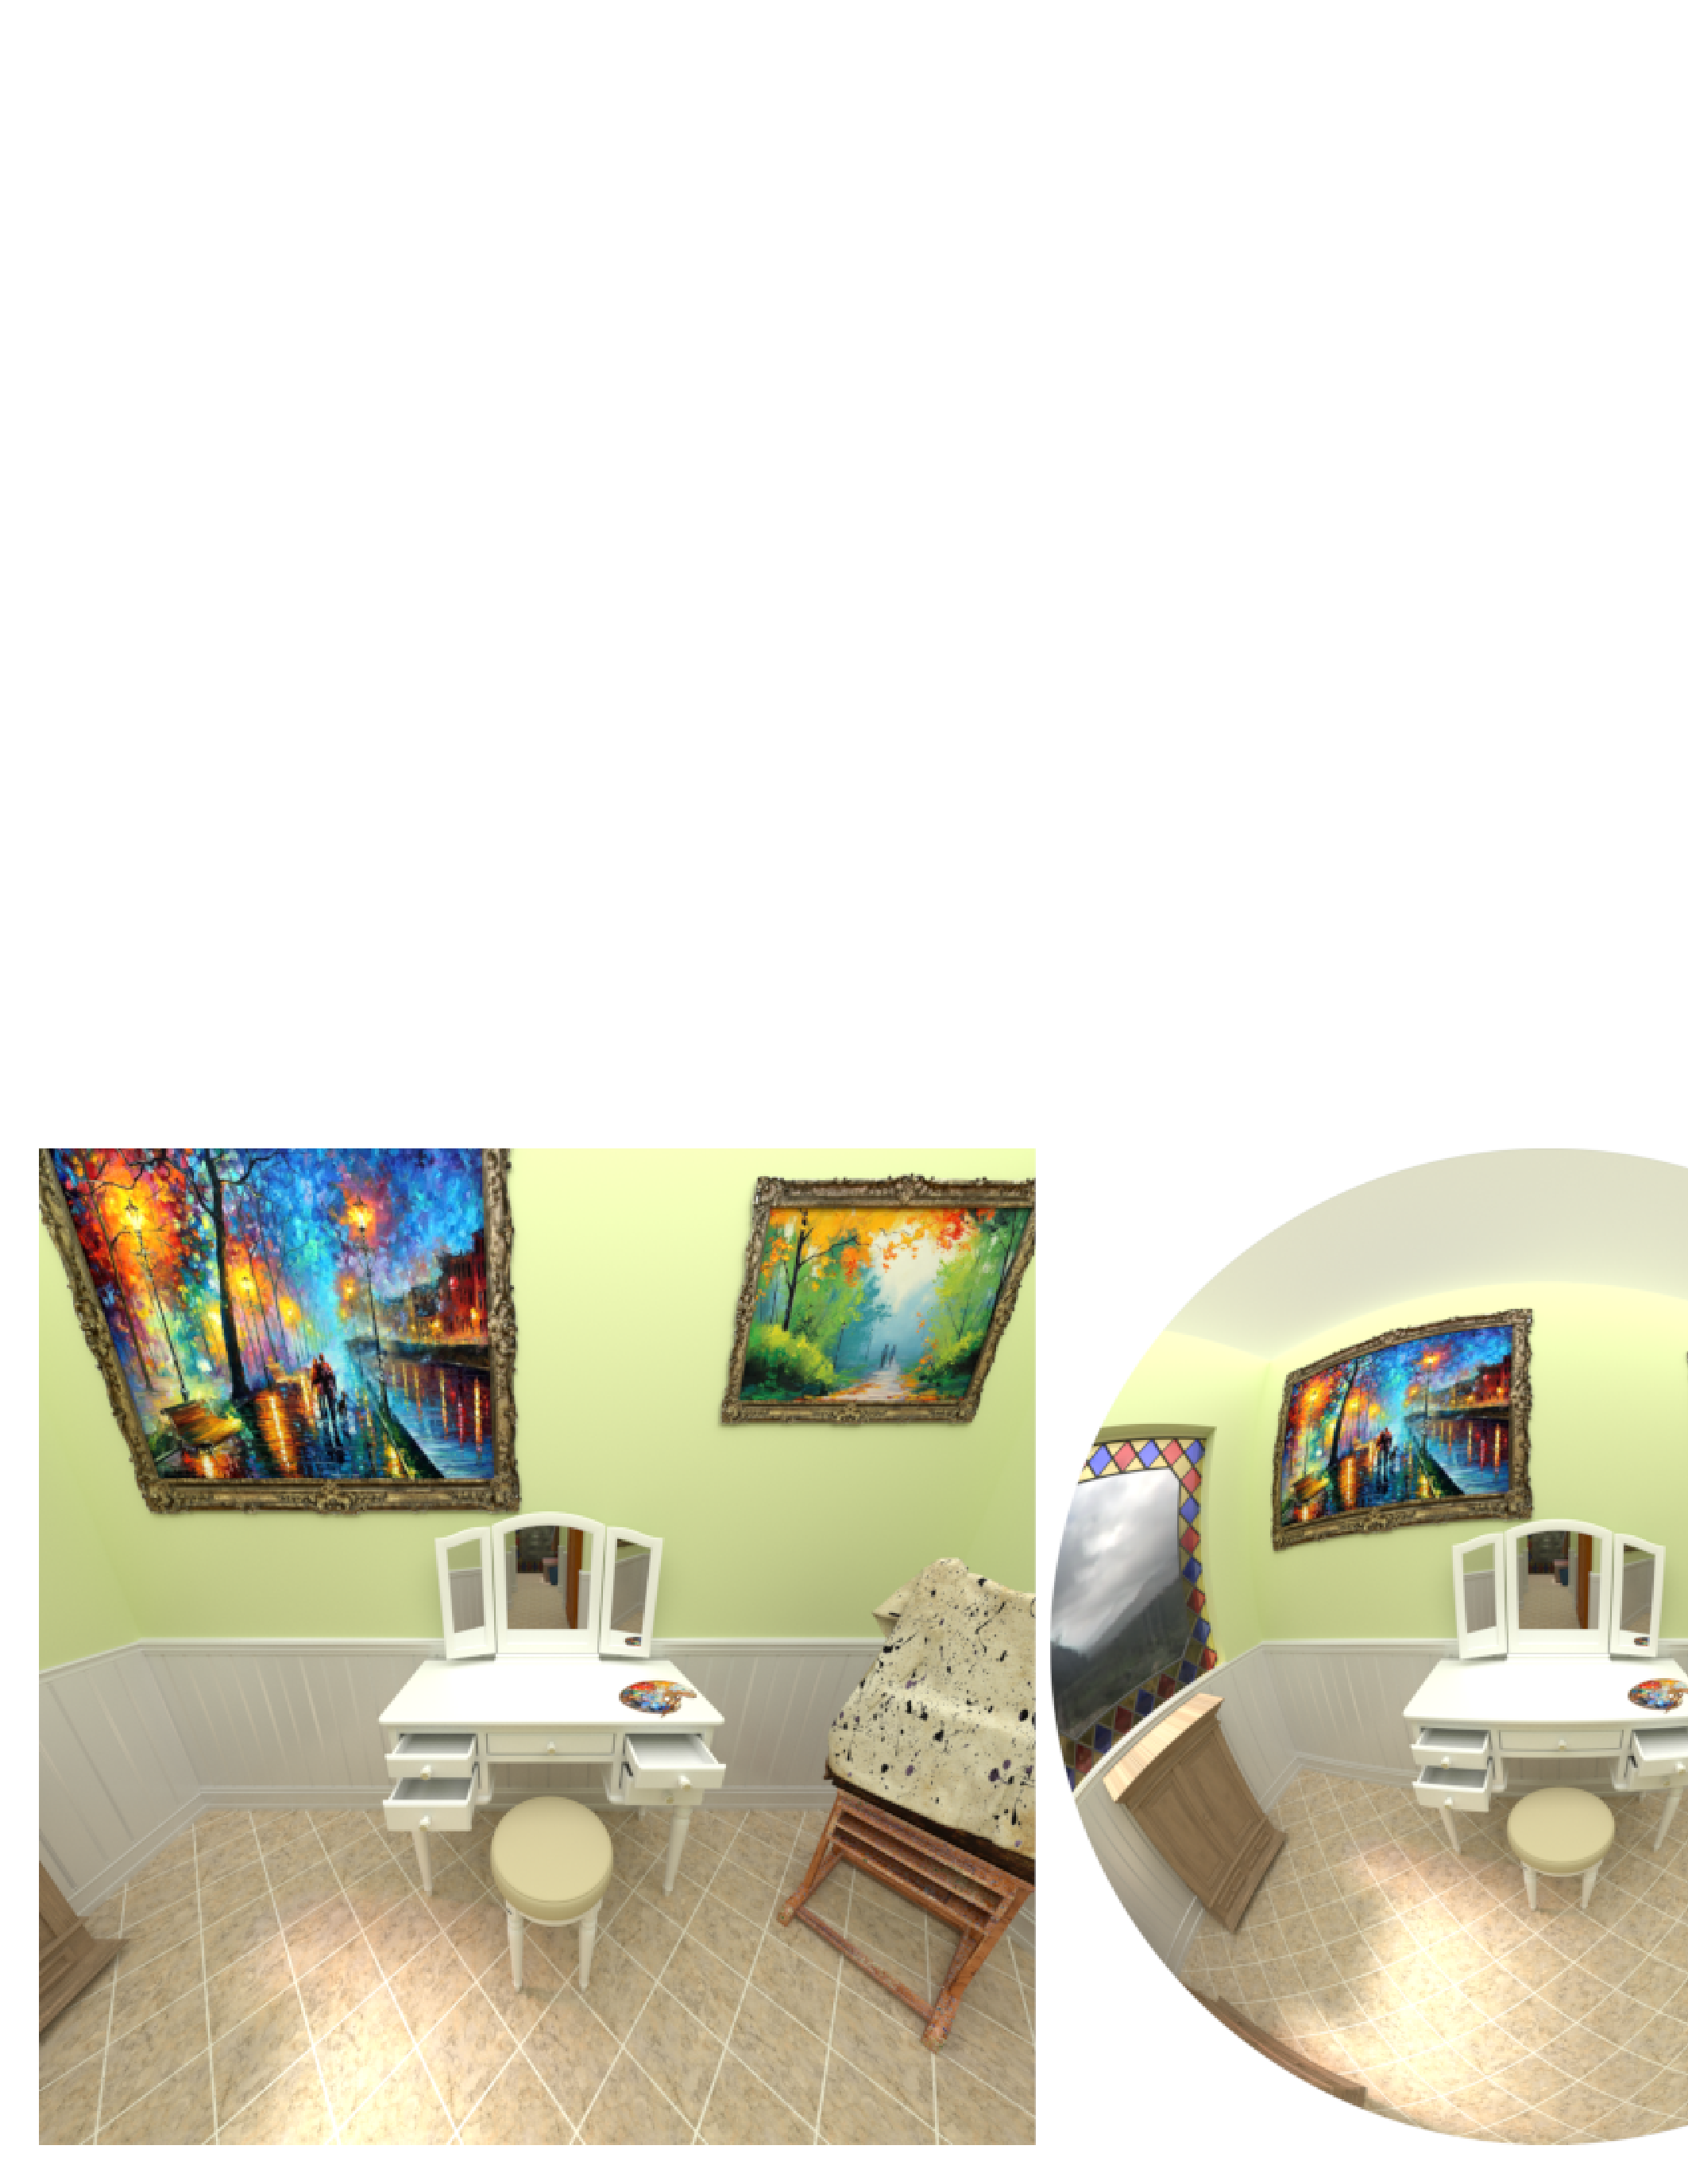}}
%\vspace{-0.2cm}
\caption{Comparison of the field of view captured by the pinhole model (left, 110$^\circ$ horizontally) and the field of view captured by the equisolid fisheye model (right, 185$^\circ$ all around). For comparison purposes, the same sensor size is assumed. ***do this with a 8mm lens?***}
\label{fig:fovcomparison}
%\vspace{-0.6cm}
\end{figure}

\begin{comment}
\begin{figure}[t]
%\small
\centering
\centerline{\includegraphics[width=1.0\columnwidth]{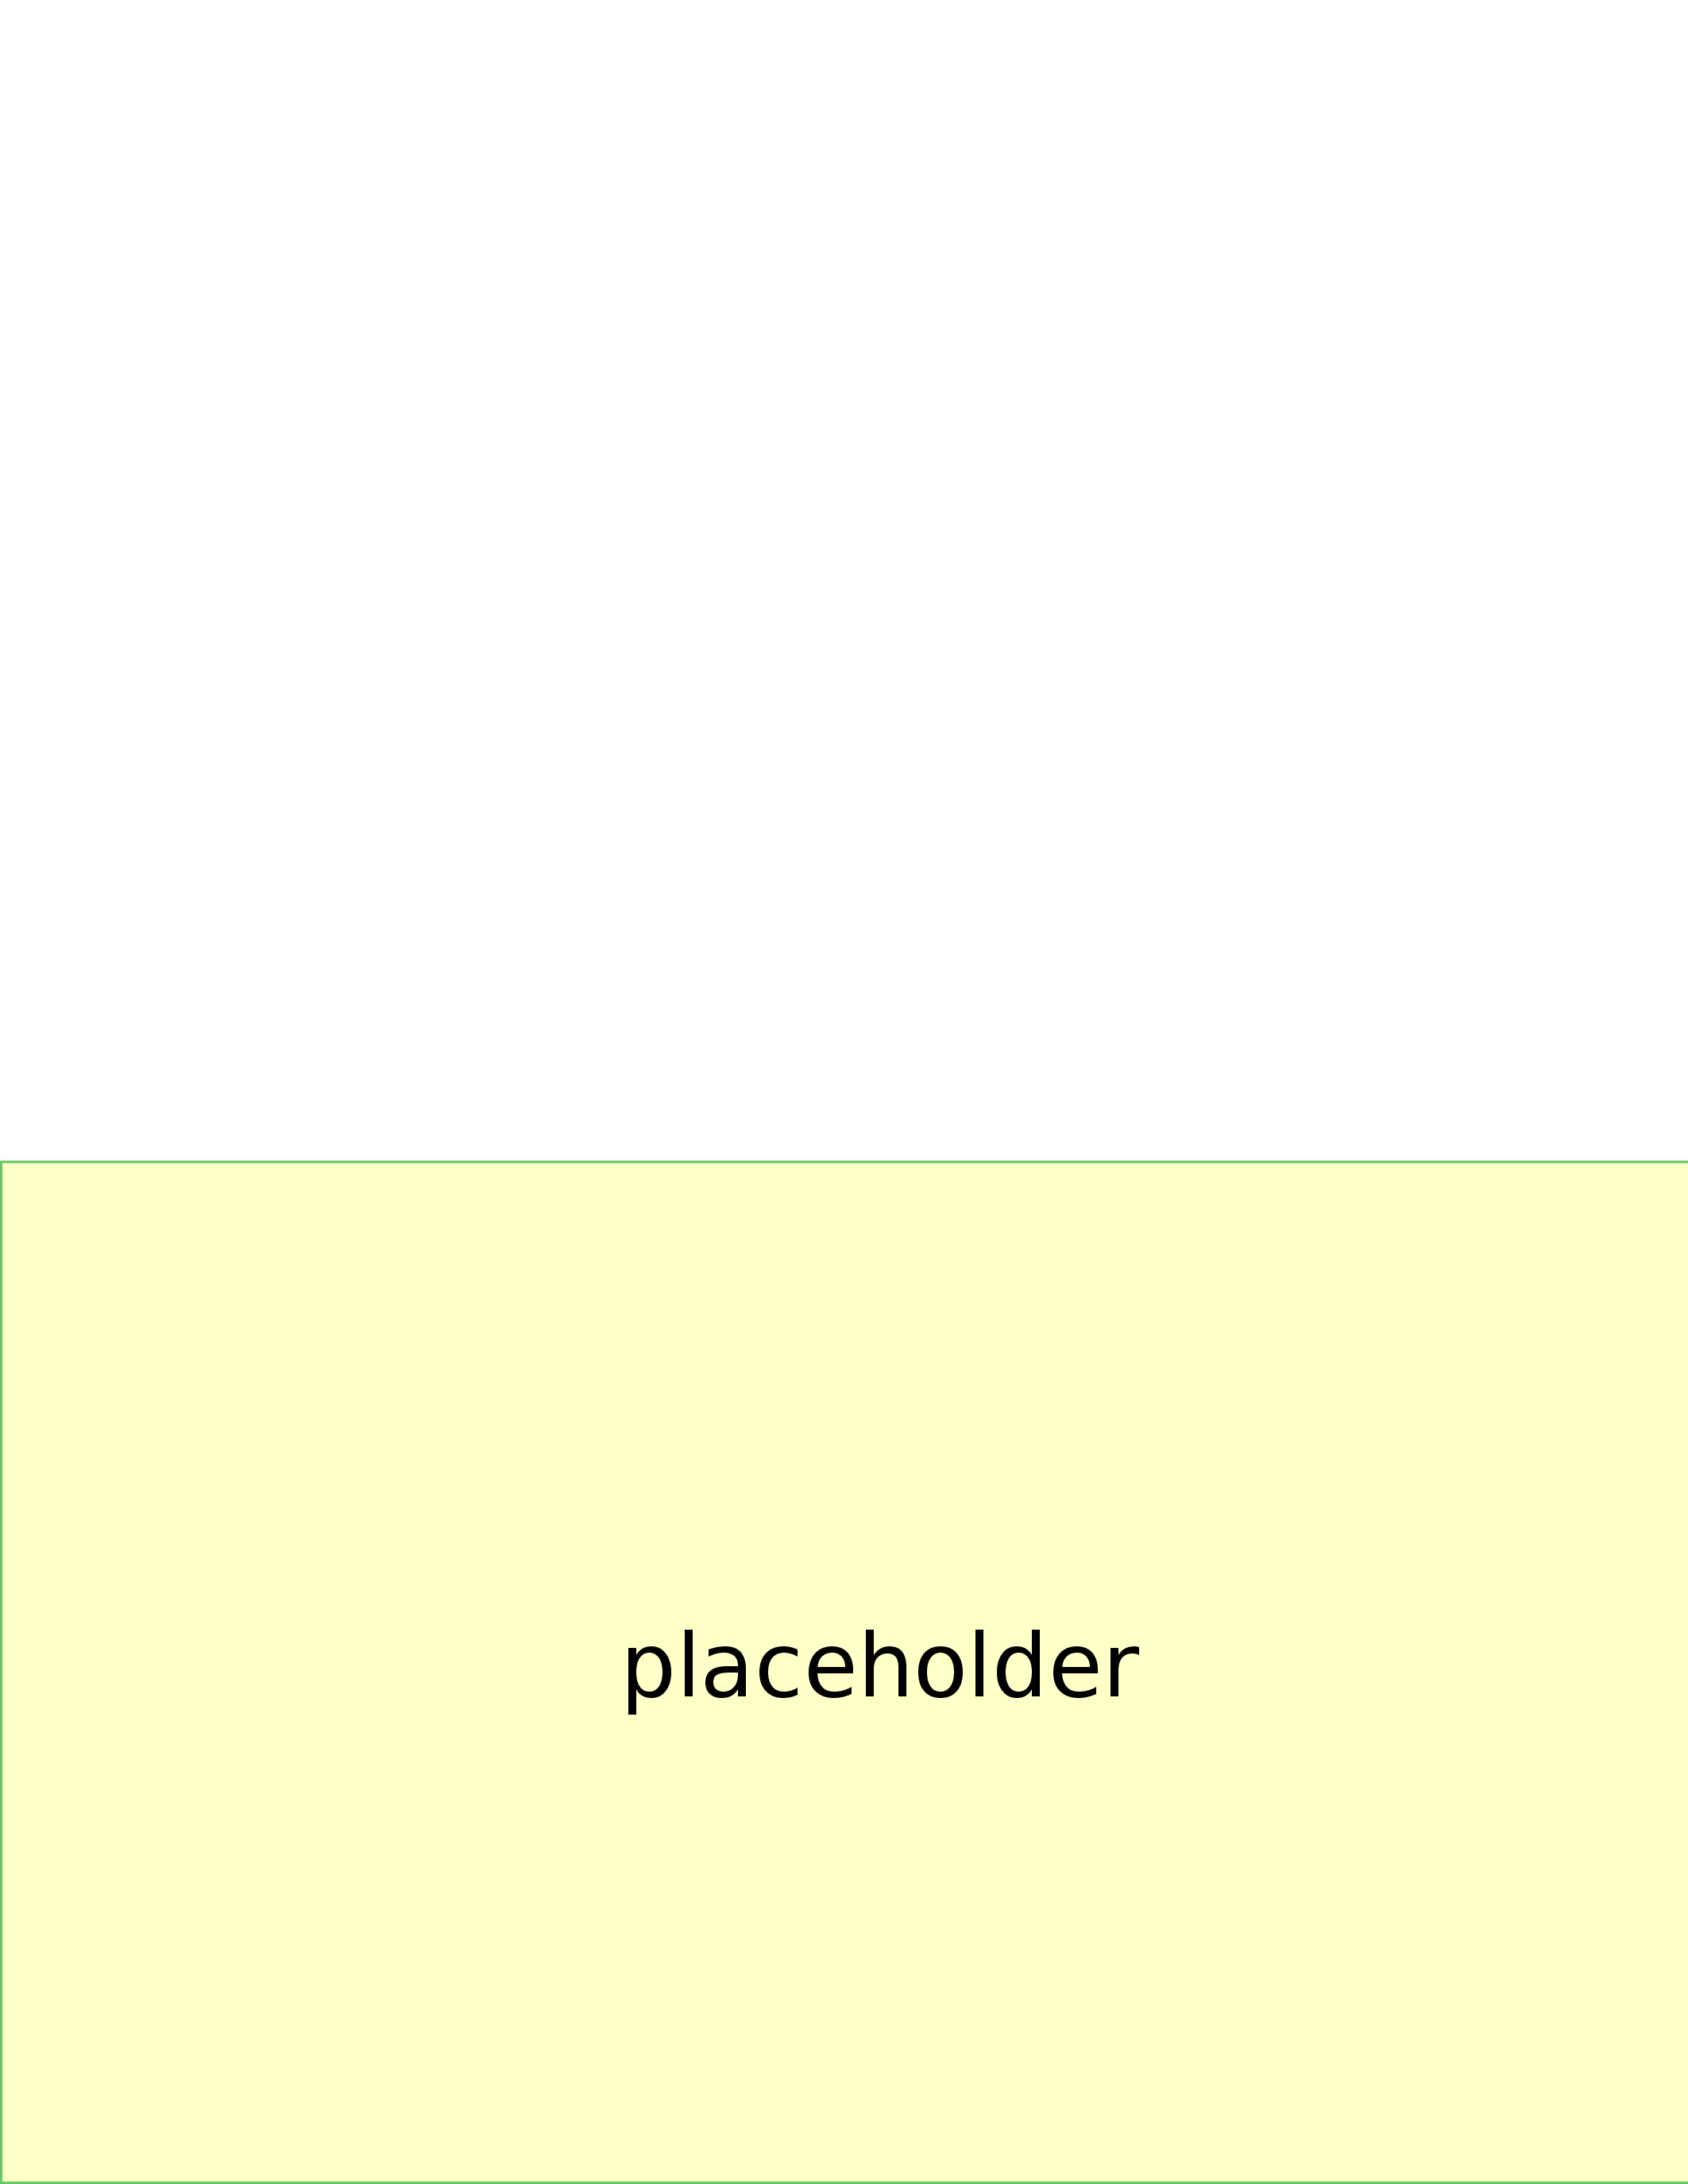}}
%\vspace{-0.2cm}
\caption{Image of camera on tripod with a focus on the lens.}
\label{fig:realimg}
%\vspace{-0.6cm}
\end{figure}

Fig.~\ref{fig:EME} illustrates the proposed method, where $\mathcal{E}$ and $\mathcal{P}$ denote what, in this paper, we call the equisolid and the perspective domain, respectively.
\begin{figure}[t]
%\small
\centering
\centerline{\includegraphics[width=0.5\columnwidth]{figures/placeholder}}
\caption{Block diagram with details of EME.}
\label{fig:EME}
\end{figure}
\end{comment}

\begin{figure}[t]
%\small
\centering
\psfrag{a}[lB][lB]{{\color[rgb]{0.5,0,0}$180^\circ$}}
\psfrag{o}[lB][lB]{{\color[rgb]{0.5,0,0}$2(\text{max}-180)$}}
\psfrag{t}[cc][cc]{{\color[rgb]{1,0.47,0}$\theta_{180}$}}
\psfrag{m}[cc][cc]{{\color[rgb]{0.61,0.61,0.61}$\theta_{\text{max}}$}}
\psfrag{d}[cc][cc]{{\color[rgb]{0.39,0.78,0.39}$\theta_{2\cdot 180-\text{max}}$}}
\centerline{\includegraphics[width=0.7\columnwidth]{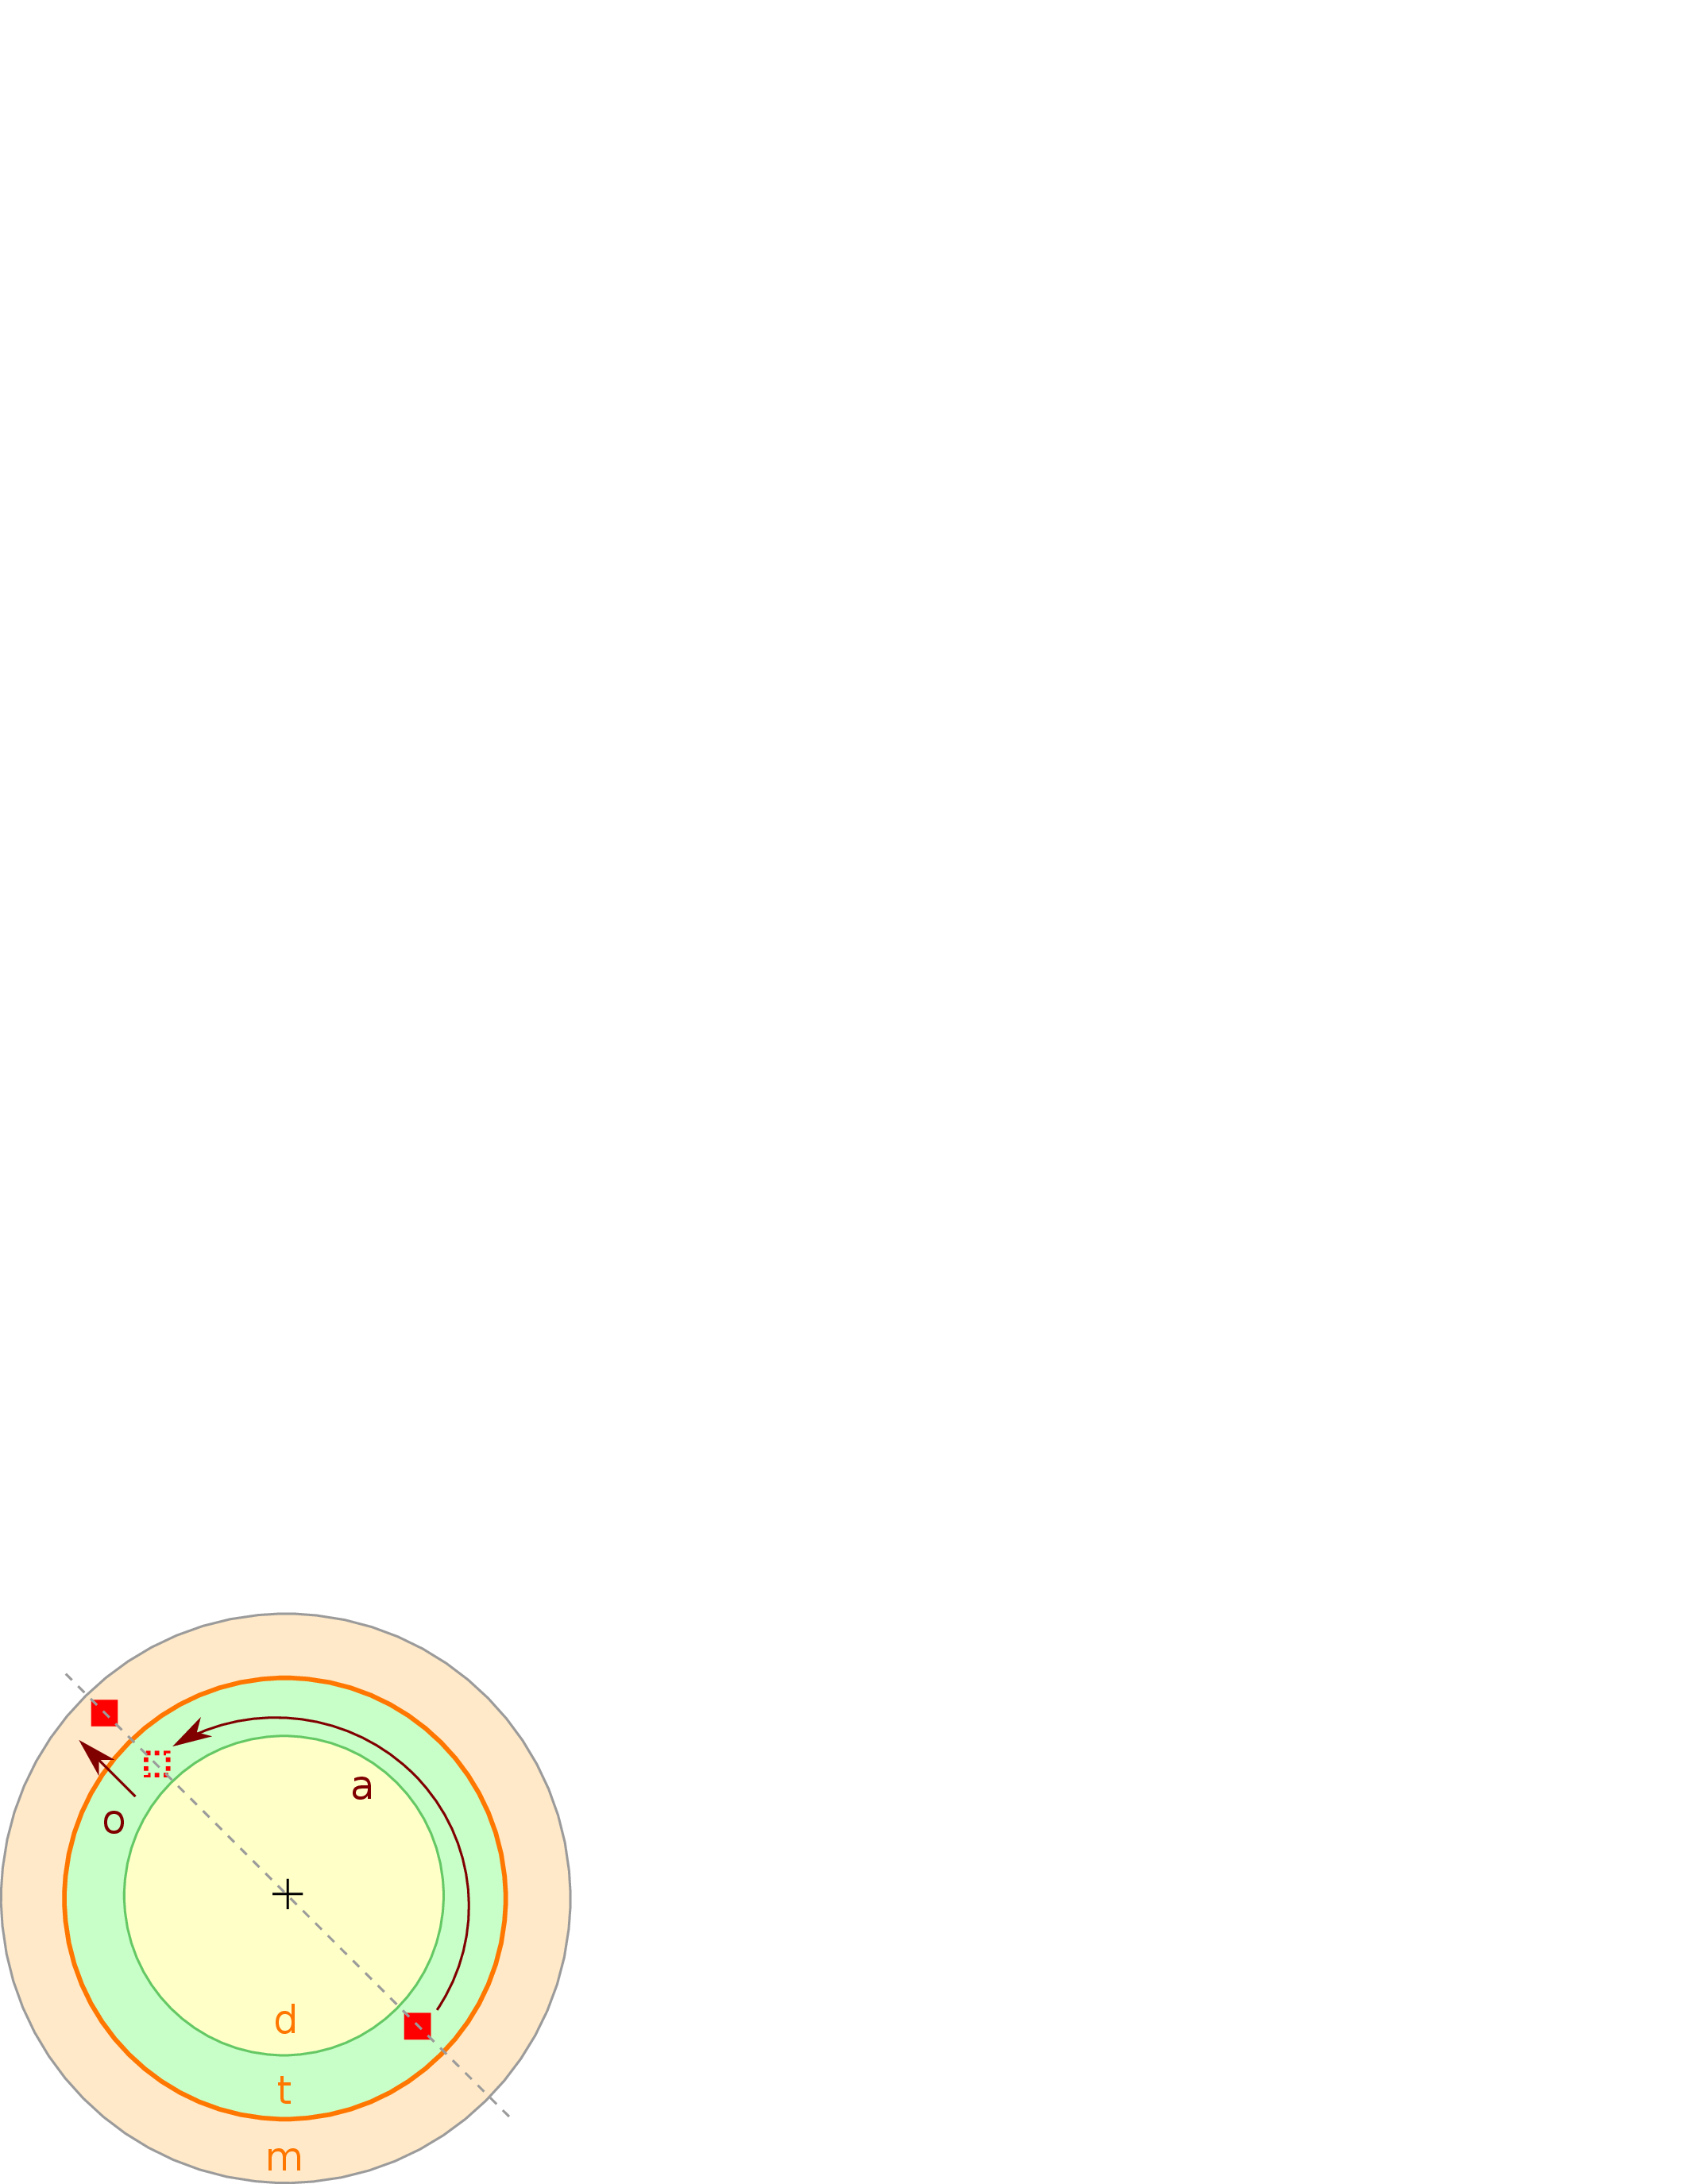}}
\caption{Schematic depiction of a fisheye image and the origin of pixels in the $\theta > 180^\circ$ area (orange) therein. Without a suitable compensation, the orange area is a mirrored and rotated version of the green area.}
\label{fig:ultrawideanglecompensation}
\end{figure}

\begin{figure}[t]
%\small
\centering
\centerline{\includegraphics[width=1.0\columnwidth]{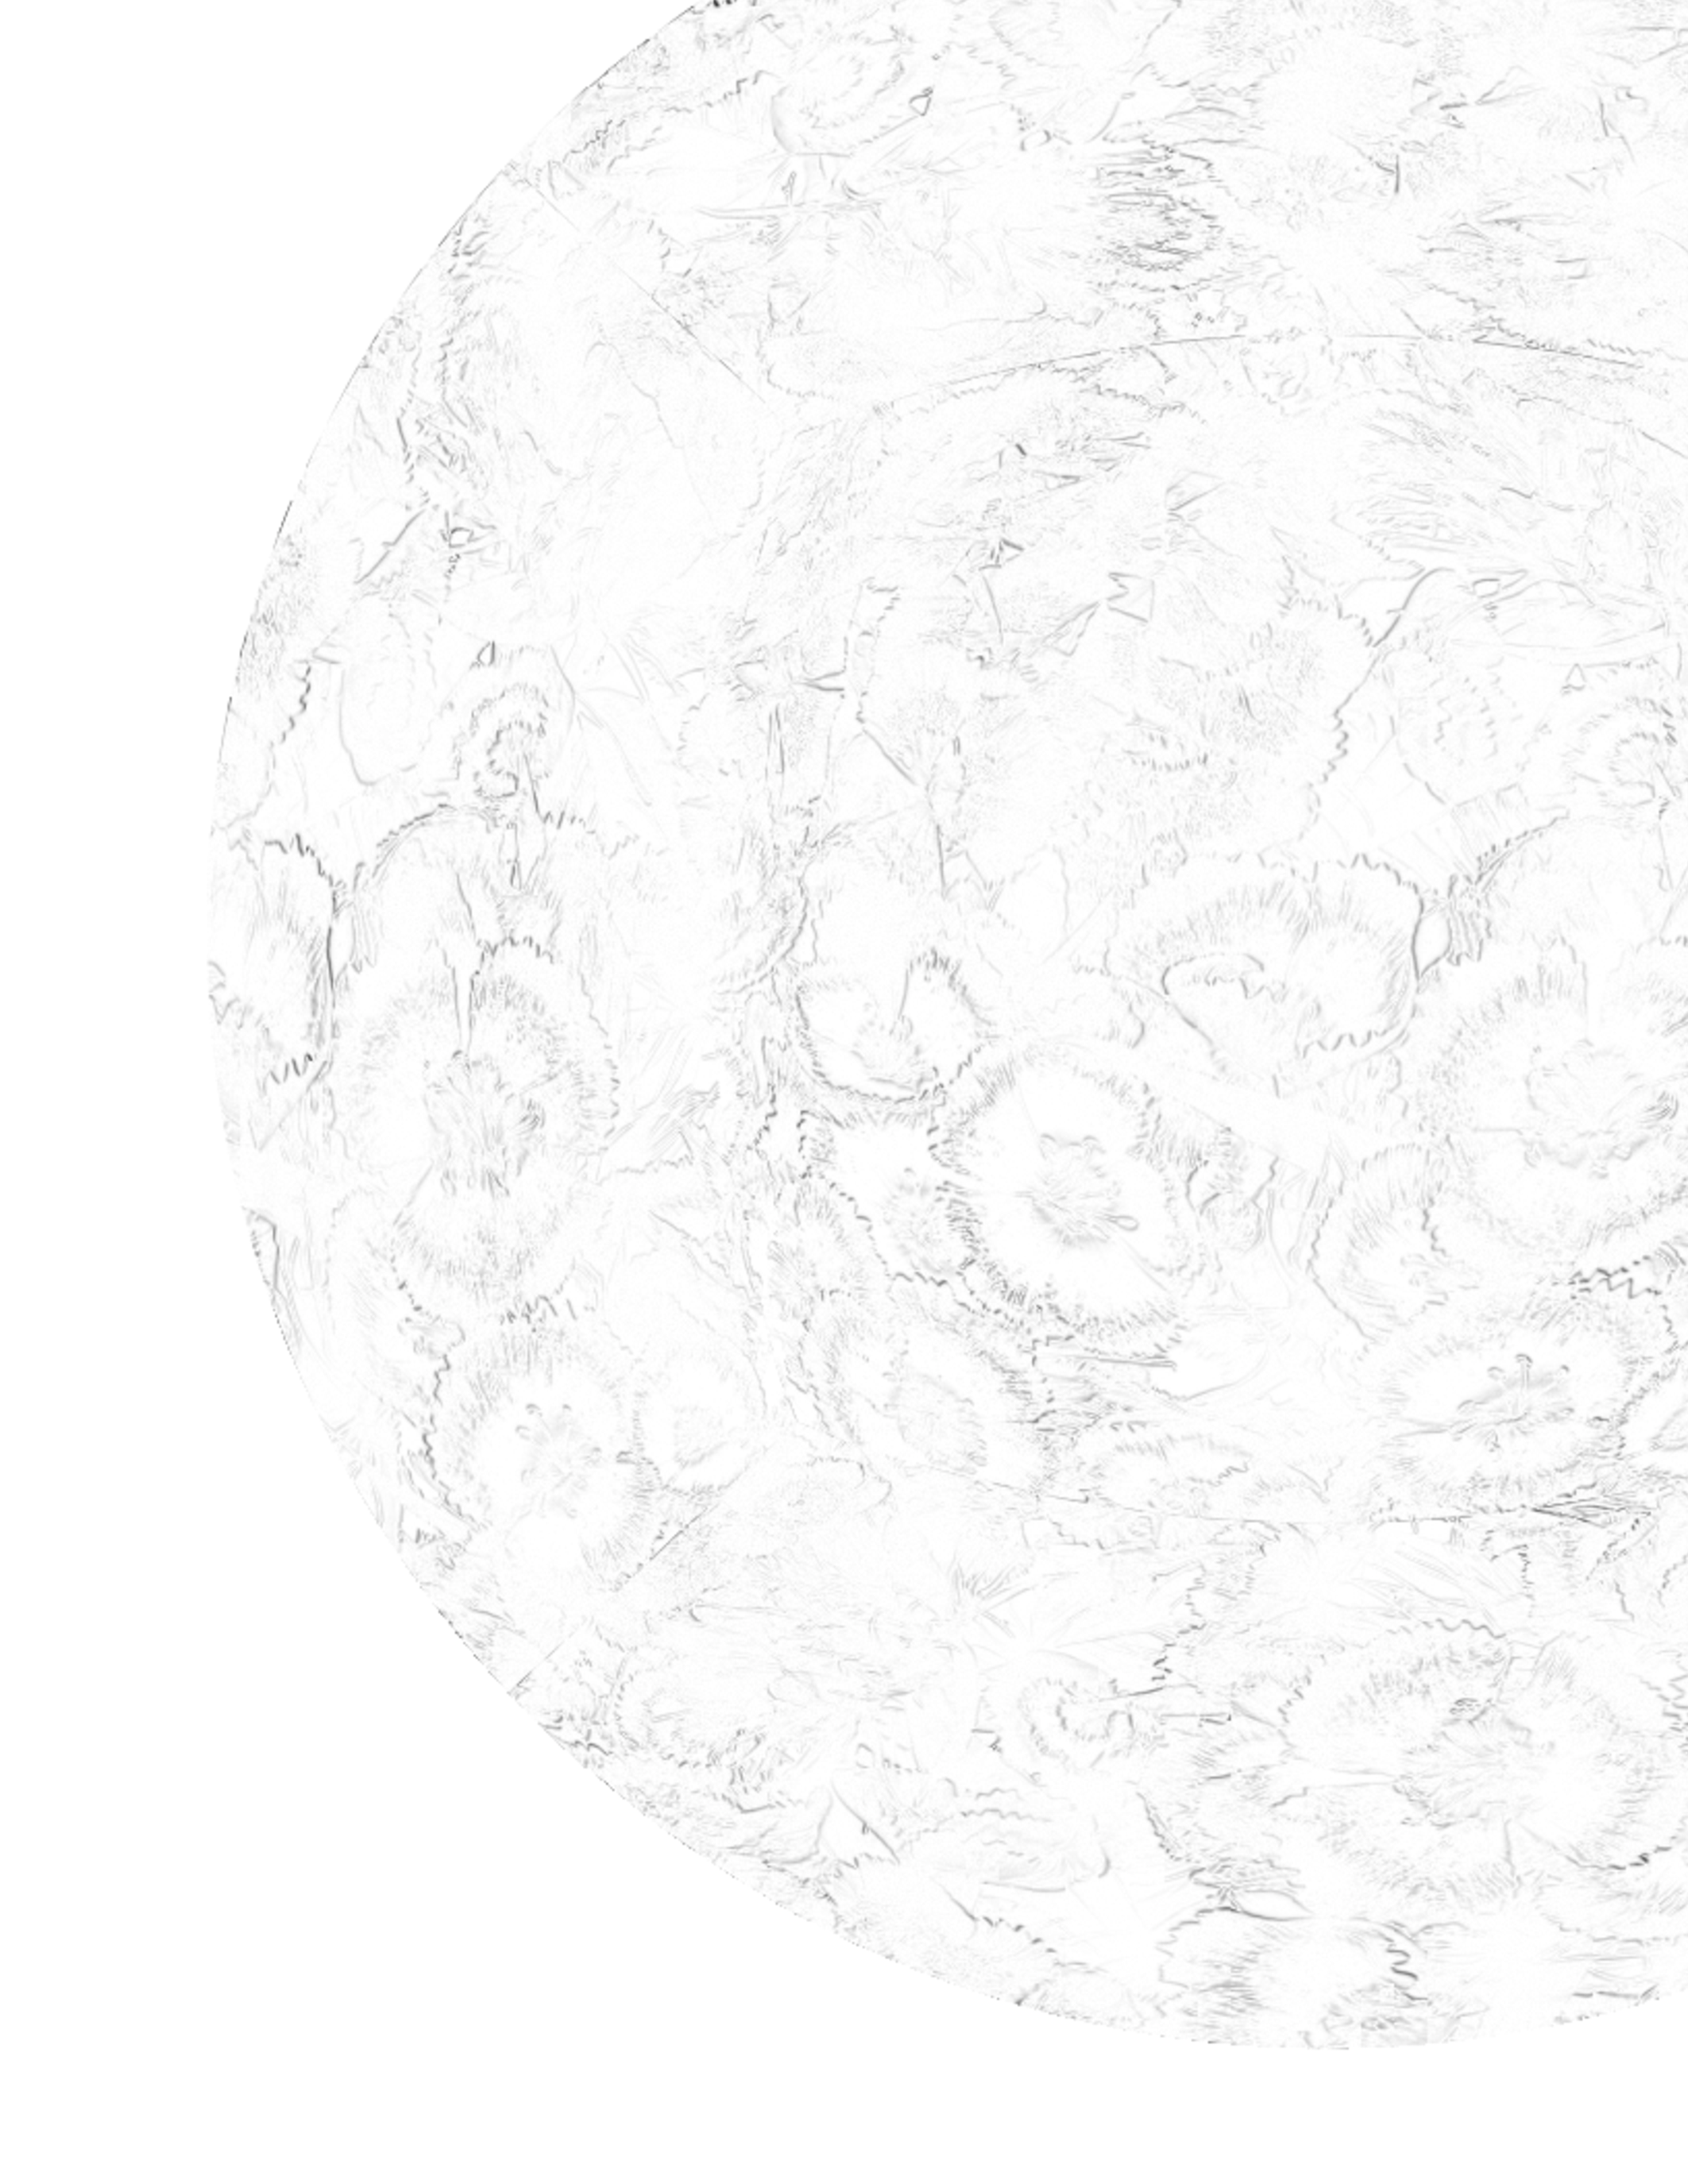}}
%\vspace{-0.2cm}
\caption{Absolute residual error signals after motion compensation via TME (left) and EME+ (right), best viewed enlarged on screen.}
\label{fig:flowersdiff}
%\vspace{-0.6cm}
\end{figure}

\begin{figure}[t]
\centering
\input{figures/equisolidterm2}
\caption{$fg(\boldsymbol{P})$.}
\end{figure}

\begin{figure*}[t]
\centering
\input{figures/motionanalysis}
\input{figures/motionanalysisgain}
\caption{[PLACEHOLDER] Effect of motion type on estimation performance. Example sequence: Clips. Frames: 5 till 345 in steps of 5. Motion changes after every 50 steps: T hor, T diag, T vert, P hor, ... Maybe replace by block size figure}
\label{fig:motionanalysis}
\end{figure*}
